# Supplementary material for: Ensemble Prediction of Time to Event Outcomes with Competing Risks: A Case Study of Surgical Complications in Crohn's Disease
Source: arXiv:1902.02533 source file (2019-02-07)
Supplement: Supplementary file 1 [file prediction-complications-inflammatory-supplement.pdf]

# Ensemble Prediction of Time to Event Outcomes with Competing Risks: A Case Study of Surgical Complications in Crohn's Disease

Michael C Sachs

*Department of Medicine, Karolinska Institutet Stockholm, Sweden.*

E-mail: michael.sachs@ki.se

Andrea Discacciati

*Institute of Environmental Medicine, Karolinska Institutet, Stockholm, Sweden.*

Åsa H Everhov

*Department of Medicine, Karolinska Institutet, Stockholm, Sweden.*

Ola Olén

*Department of Medicine, Karolinska Institutet, Stockholm, Sweden.*

Erin E Gabriel

*Department of Medical Epidemiology and Biostatistics, Karolinska Institutet, Stockholm, Sweden.*

## 1. SUPPLEMENTARY MATERIAL

### *1.1. Additional Simulation Results*

We simulated one replicate from the interaction with the crossing effect as described by Goldstein et al. (2015). Specifically we generate data where there are only two variables, X1 and X2, where X1 in continuous and X2 is binary. There is an interaction effect such that when X2 equals 0, the association between X1 and Y is positive and linear, and when X2 equals 1, the association is negative and linear. The association between these variables and the true probability of the outcome is shown in Figure 1. We simulated data from this scenario, fit a superlearner model on the pseudo observations, and then

ran both the PDP and the perturbation algorithms.

As expected, the PDP plot for variable X1 shows that there is no association with the outcome (Figure 2). However, we see from our perturbation algorithm plot, that the local slopes appear to be different from 0 for that variable, suggesting that our approach, to some degree, alleviates one of the main criticisms of the PDP plot.

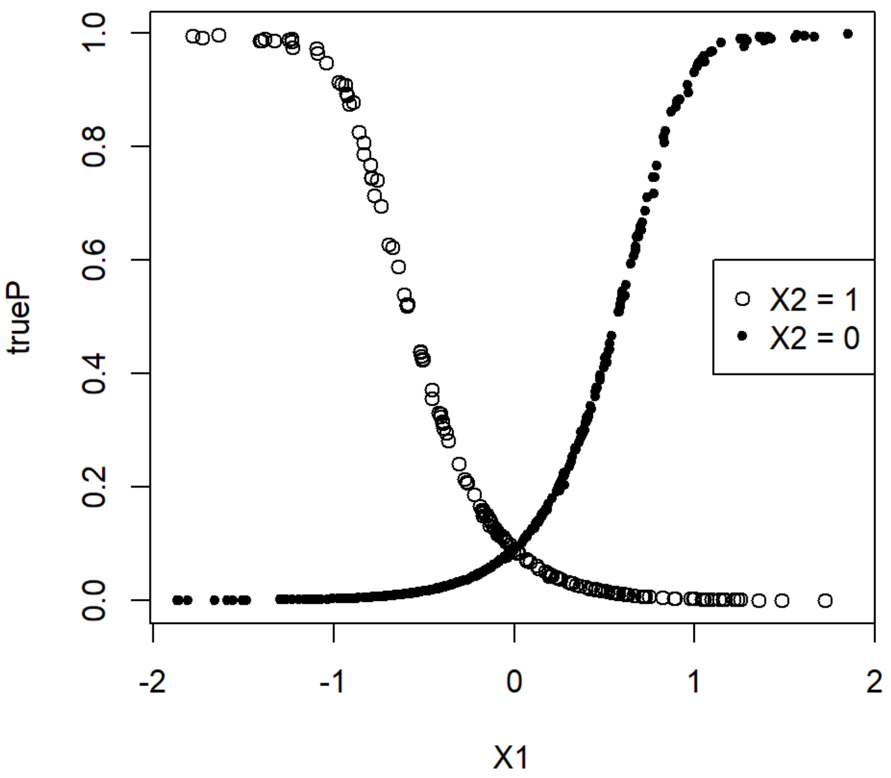


**Fig. 1.** Simulated crossing interaction scenario used to evaluate the PDP and perturbation algorithms.

### *1.2. Description of Study Population*

**Table 1.** Abbreviations for variables used in the data analysis.

| Abbreviation | Description |
|---|---|
| age_ibd1 | Age at CD onset |
| male | Male gender |
| inpatient | CD diagnosed as inpatient |
| year_ibd1 | Year of CD onset |
| immunomodulators | Dispensed immunomodulators |
| antiTNF | Dispensed tumor necrosis factor inhibitors |
| infliximab | Dispensed infliximab |
| cstd | Dispensed corticosteroids |
| loccstd | Dispensed locally acting steroids |
| rekasa | Dispensed rectal ASA |
| sysasa | Dispensed systemic ASA |
| antibiot | Dispensed IBD antibiotics |
| EIM | Extraintestinal manifestations |
| PSC | Primary sclerosing cholangitis |
| relative_has_UC | First degree relative has Ulcerative colitis |
| relative_has_CD | First degree relative has CD |
| diab | Diabetes |
| hyp | Hypertension |
| ihd | Ischemic heart disease |
| cervd | Cererbrovascular disease |
| chd | Congestive heart disease |
| copd | Chronic obstructive pulmonary disorder |
| kfail | Kidney failure |
| maxeduc | Highest parental education (scale from 1 to 7) |
| immigrantmom | Mother born outside of Sweden |
| immigrant | Patient born outside of Sweden |
| parisB1 | Montreal/Paris B1: non stricturing/non penetrating |
| parisL3 | Montreal/Paris L3: Ileocecal/location not defined |
| parisP.plus | Montreal/Paris P+: Perianal disease |

**Table 2.** Description of study population and potential predictors. Demographics and family characteristics.

| | Censored (n=10827) | Died (n=1508) | Surgery (n=3027) | Overall (n=15362) |
|---|---|---|---|---|
| **Age at onset** | | | | |
| Mean (SD) | 40.3 (16.1) | 64.6 (17.9) | 41.3 (17.3) | 42.8 (18.0) |
| Median [Min, Max] | 37.4 [18.0, 93.4] | 69.5 [18.2, 97.8] | 38.2 [18.0, 91.4] | 39.8 [18.0, 97.8] |
| Male | 5047 (46.6%) | 693 (46.0%) | 1487 (49.1%) | 7227 (47.0%) |
| Female | 5780 (53.4%) | 815 (54.0%) | 1540 (50.9%) | 8135 (53.0%) |
| **Inpatient** | | | | |
| Yes | 3559 (32.9%) | 926 (61.4%) | 1730 (57.2%) | 6215 (40.5%) |
| No | 7268 (67.1%) | 582 (38.6%) | 1297 (42.8%) | 9147 (59.5%) |
| **Onset year** | | | | |
| Mean (SD) | 2010 (5.80) | 2000 (5.99) | 2000 (6.26) | 2000 (6.18) |
| **Highest parental education** | | | | |
| Primary school | 1971 (18.2%) | 171 (11.3%) | 609 (20.1%) | 2751 (17.9%) |
| Secondary school | 524 (4.8%) | 24 (1.6%) | 166 (5.5%) | 714 (4.6%) |
| Upper secondary school 2 years | 2631 (24.3%) | 71 (4.7%) | 673 (22.2%) | 3375 (22.0%) |
| Upper secondary school 3 years | 3378 (31.2%) | 1177 (78.1%) | 1031 (34.1%) | 5586 (36.4%) |
| University < 3 years | 1013 (9.4%) | 28 (1.9%) | 236 (7.8%) | 1277 (8.3%) |
| University 3 years or more | 1215 (11.2%) | 34 (2.3%) | 297 (9.8%) | 1546 (10.1%) |
| Post graduate | 95 (0.9%) | 3 (0.2%) | 15 (0.5%) | 113 (0.7%) |
| **Mother born outside Sweden** | 1211 (11.2%) | 73 (4.8%) | 281 (9.3%) | 1565 (10.2%) |
| **Born outside Sweden** | 1522 (14.1%) | 257 (17.0%) | 391 (12.9%) | 2170 (14.1%) |

**Table 3.** Description of study population and potential predictors. Medications and IBD characteristics.

| | Censored (n=10827) | Died (n=1508) | Surgery (n=3027) | Overall (n=15362) |
|---|---|---|---|---|
| **Immunomodulators** | 1218 (11.2%) | 50 (3.3%) | 146 (4.8%) | 1414 (9.2%) |
| **anti-TNF** | 118 (1.1%) | 1 (0.1%) | 13 (0.4%) | 132 (0.9%) |
| **Infliximab** | 46 (0.4%) | 1 (0.1%) | 4 (0.1%) | 51 (0.3%) |
| **Corticosteroids** | 3354 (31.0%) | 216 (14.3%) | 530 (17.5%) | 4100 (26.7%) |
| **Local steroids** | 1847 (17.1%) | 93 (6.2%) | 312 (10.3%) | 2252 (14.7%) |
| **Rectal ASA** | 2229 (20.6%) | 122 (8.1%) | 246 (8.1%) | 2597 (16.9%) |
| **Systemic ASA** | 2641 (24.4%) | 145 (9.6%) | 295 (9.7%) | 3081 (20.1%) |
| **Antibiotics** | 2073 (19.1%) | 166 (11.0%) | 411 (13.6%) | 2650 (17.3%) |
| **Extraintestinal manifestations** | 268 (2.5%) | 25 (1.7%) | 47 (1.6%) | 340 (2.2%) |
| **Primary Sclerosing Cholangitis** | 57 (0.5%) | 17 (1.1%) | 10 (0.3%) | 84 (0.5%) |
| **Relative has UC** | 722 (6.7%) | 38 (2.5%) | 219 (7.2%) | 979 (6.4%) |
| **Relative has CD** | 877 (8.1%) | 37 (2.5%) | 278 (9.2%) | 1192 (7.8%) |
| **Stricturing/penetrating** | 1005 (9.3%) | 294 (19.5%) | 328 (10.8%) | 1627 (10.6%) |
| **Ileocecal location** | 4433 (40.9%) | 605 (40.1%) | 1127 (37.2%) | 6165 (40.1%) |
| **Perianal disease** | 582 (5.4%) | 31 (2.1%) | 179 (5.9%) | 792 (5.2%) |

**Table 4.** Description of study population and potential predictors. Comorbidities.

| | Censored (n=10827) | Died (n=1508) | Surgery (n=3027) | Overall (n=15362) |
|---|---|---|---|---|
| **Diabetes** | 372 (3.4%) | 186 (12.3%) | 89 (2.9%) | 647 (4.2%) |
| **Hypertension** | 754 (7.0%) | 357 (23.7%) | 179 (5.9%) | 1290 (8.4%) |
| **Ischemic heart disease** | 346 (3.2%) | 328 (21.8%) | 93 (3.1%) | 767 (5.0%) |
| **Cerebrovascular disease** | 158 (1.5%) | 172 (11.4%) | 49 (1.6%) | 379 (2.5%) |
| **Congestive heart disease** | 122 (1.1%) | 239 (15.8%) | 42 (1.4%) | 403 (2.6%) |
| **COPD** | 138 (1.3%) | 136 (9.0%) | 38 (1.3%) | 312 (2.0%) |
| **Kidney failure** | 131 (1.2%) | 106 (7.0%) | 27 (0.9%) | 264 (1.7%) |

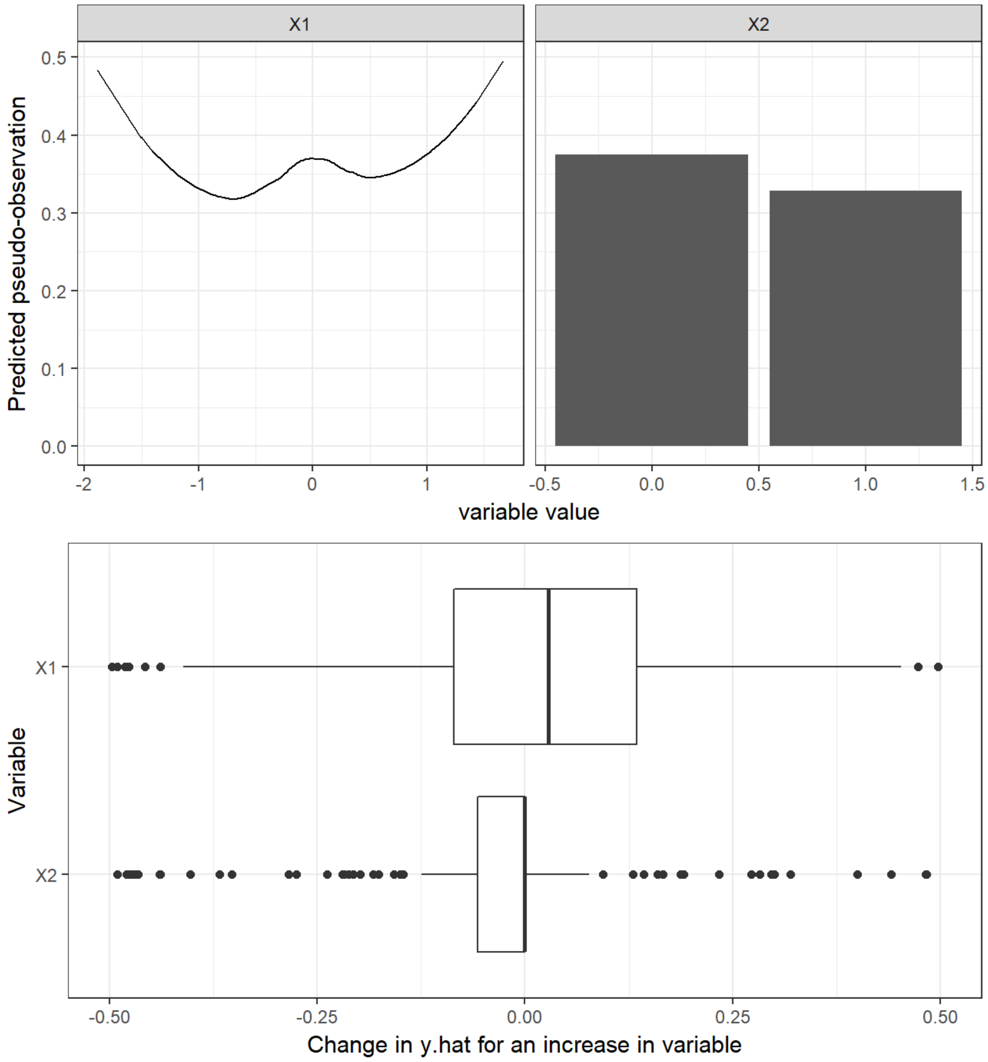


**Fig. 2.** Comparison of the PDP (top panels) and our proposed perturbation algorithm (lower panel) for the crossing interaction scenario.

### *1.3. R-code for data analysis and simulations:*

http://github.com/sachsmc/pseupersims

## 2. Bibliography

### References

Goldstein, A., Kapelner, A., Bleich, J. and Pitkin, E. (2015) Peeking inside the black box: Visualizing statistical learning with plots of individual conditional expectation. *Journal of Computational and Graphical Statistics*, **24**, 44–65.
